# Supplementary material for: Ball-Larus Path Profiling Across Multiple Loop iterations
Source: arXiv:1304.5197 source file (2013-04-18)
Supplement: Supplementary file 1 [file appendix.tex]

% !TEX root = paper.tex
%--------------------------------------------------------------------------------

\clearpage
\onecolumn
\appendix

\section{Appendix}
\label{se:appendix}

In this appendix we report further charts that will be added in the journal version of this paper.

\begin{figure*}[h]
\centerline{\includegraphics[width=0.99\textwidth]{charts/nodes-ratio-bb.eps}}
\caption{Space blowup of \kblpp\ relative to \blpp.}
\label{fig:benchmarks-space-ratio}
\end{figure*}

\begin{figure*}[h]
\centerline{\includegraphics[width=0.99\textwidth]{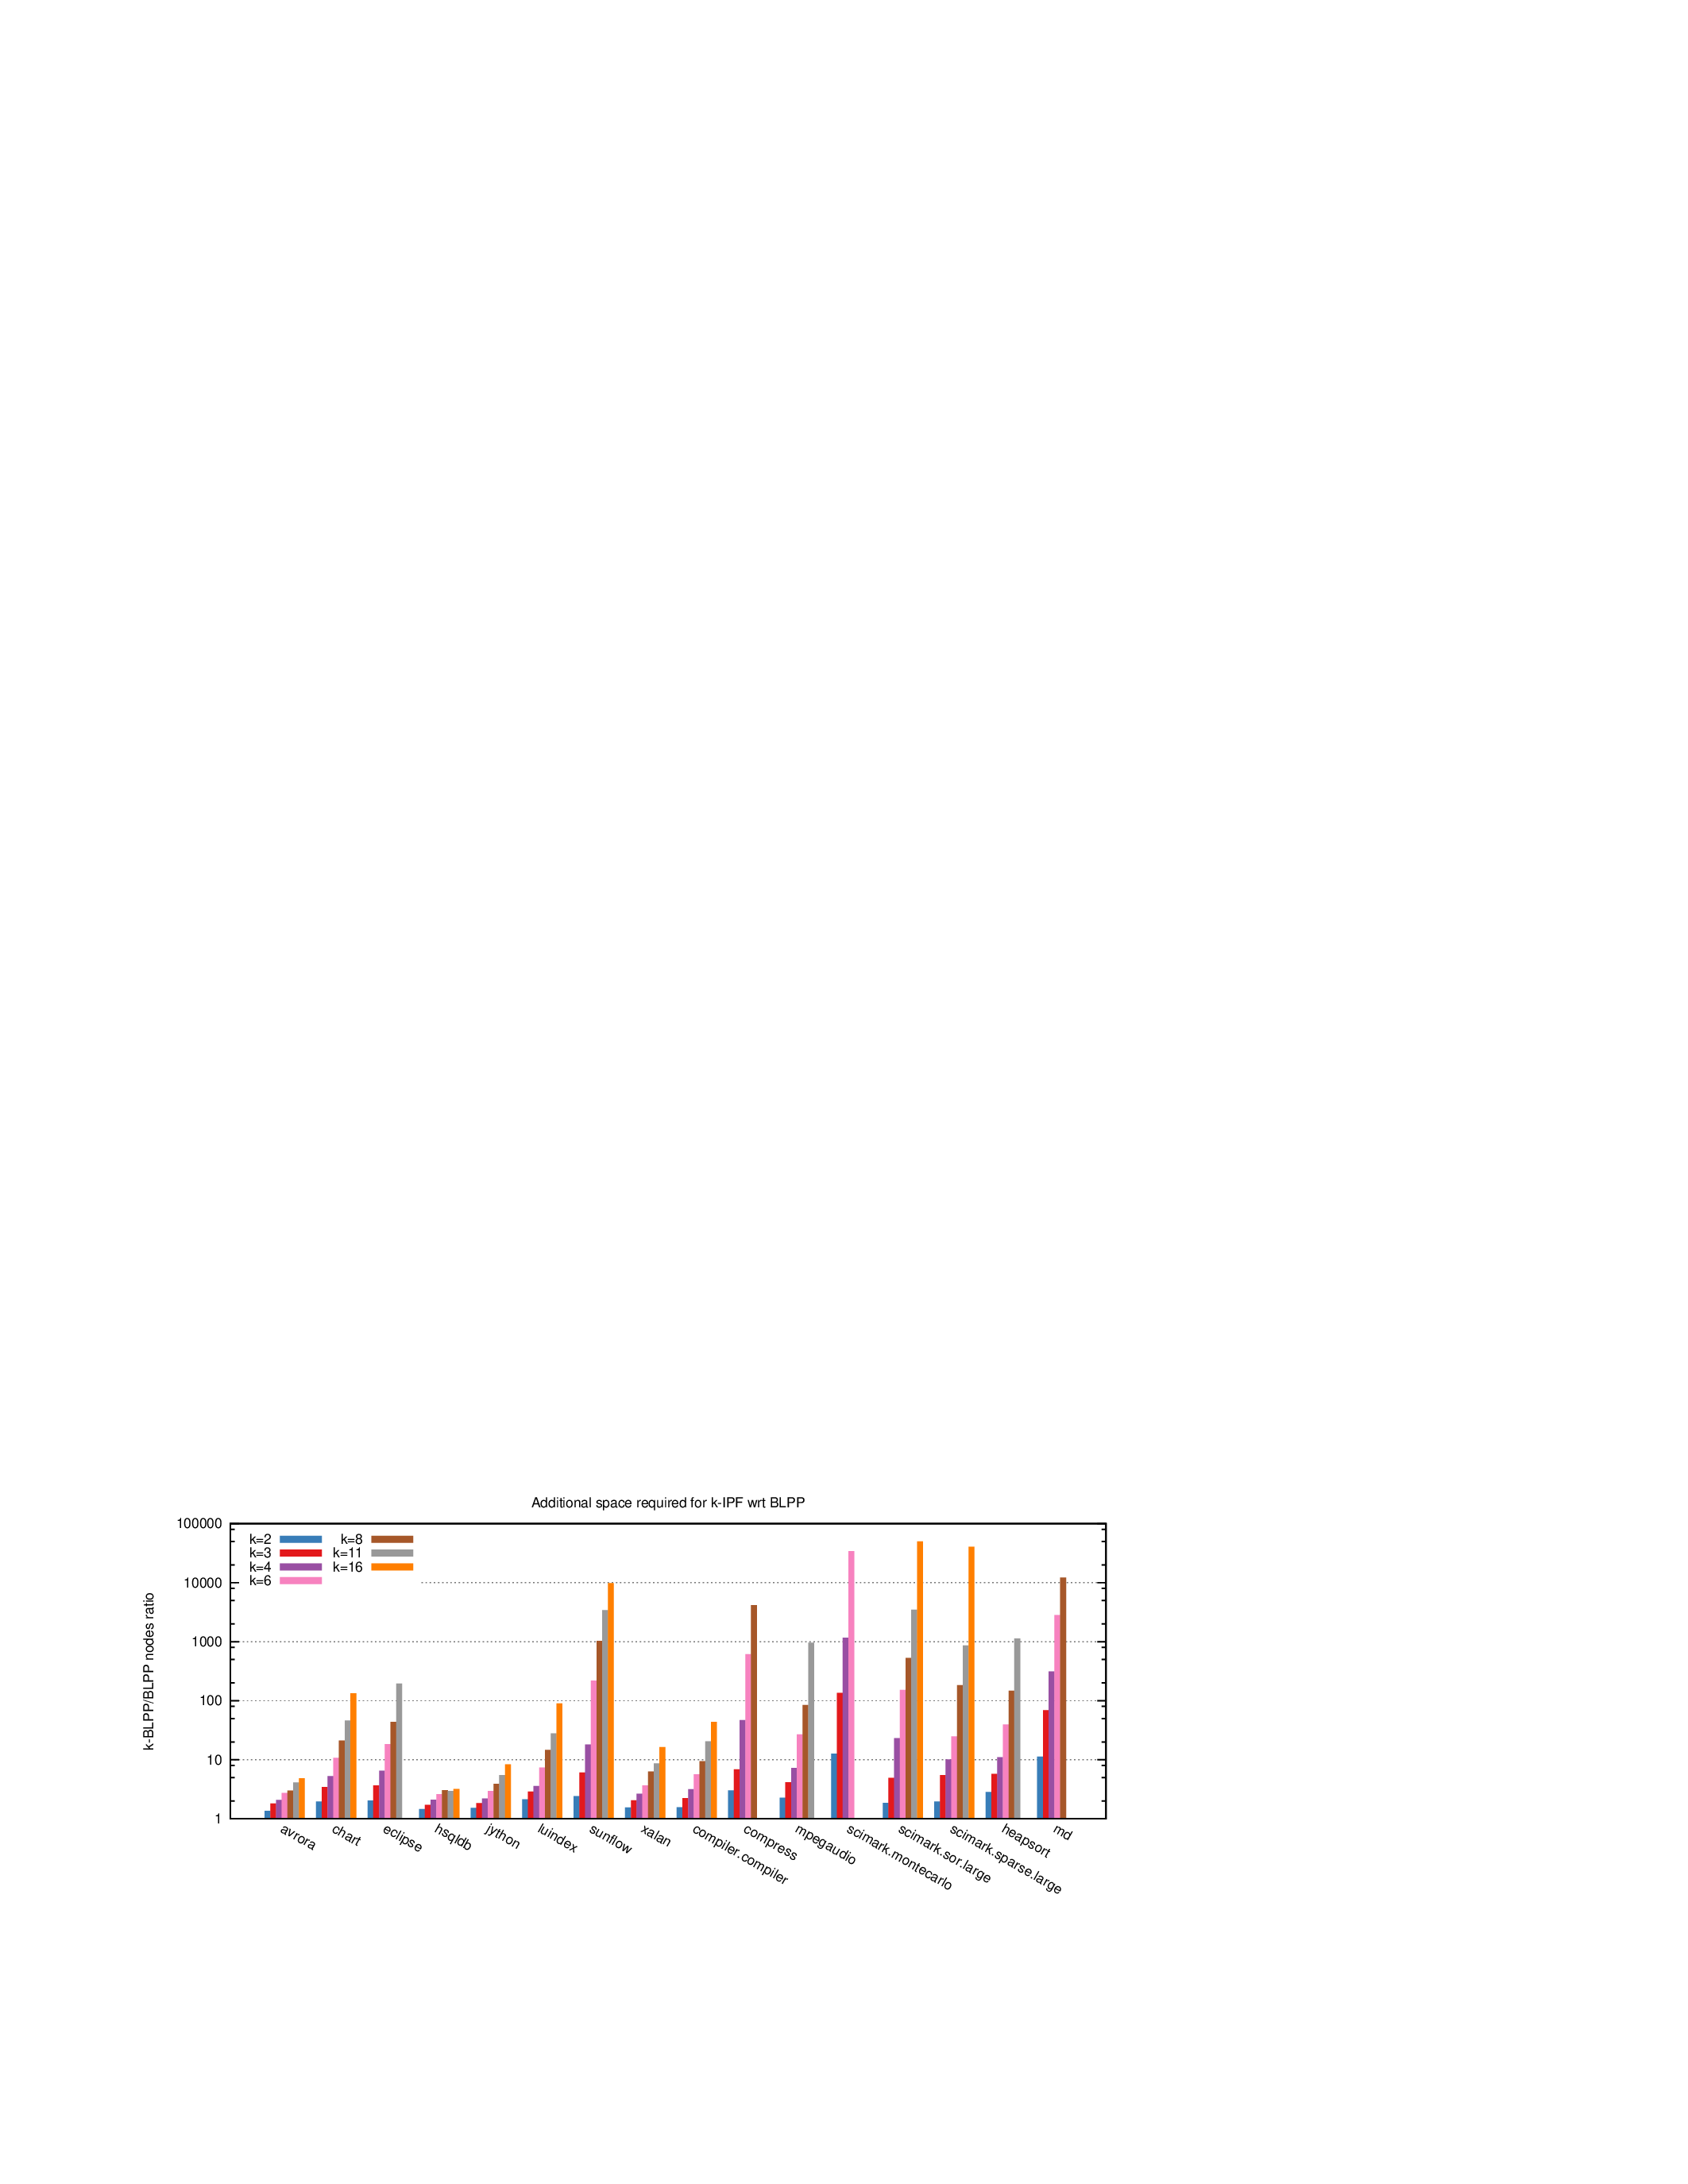}}
\caption{Profiled paths blowup of \kblpp\ relative to \blpp.}
\label{fig:benchmarks-ipf-nodes-ratio}
\end{figure*}
